# Supplementary material for: A search for top squarks with R-parity-violating decays to all-hadronic final states with the ATLAS detector in $\sqrt{s}$ = 8 TeV proton-proton collisions
Source: arXiv:1601.07453 source file (2016-06-22)
Supplement: Supplementary file 1 [file sec-appendix-aux.tex]

\subsection{Signal systematic uncertainties in each of the mass windows}
\input{tab-syst-signal.tex}

\subsection{Signal contribution in the sidebands}
\input{tab-contamination-signal.tex}

\newpage

\subsection{\ttbar \ contribution in the sidebands}
\input{tab-contamination-ttbar.tex}

\subsection{Signal efficiency for each selection}
%---------------------
\begin{figure}[!ht]
    \centering
     \includegraphics[width=0.9\columnwidth]{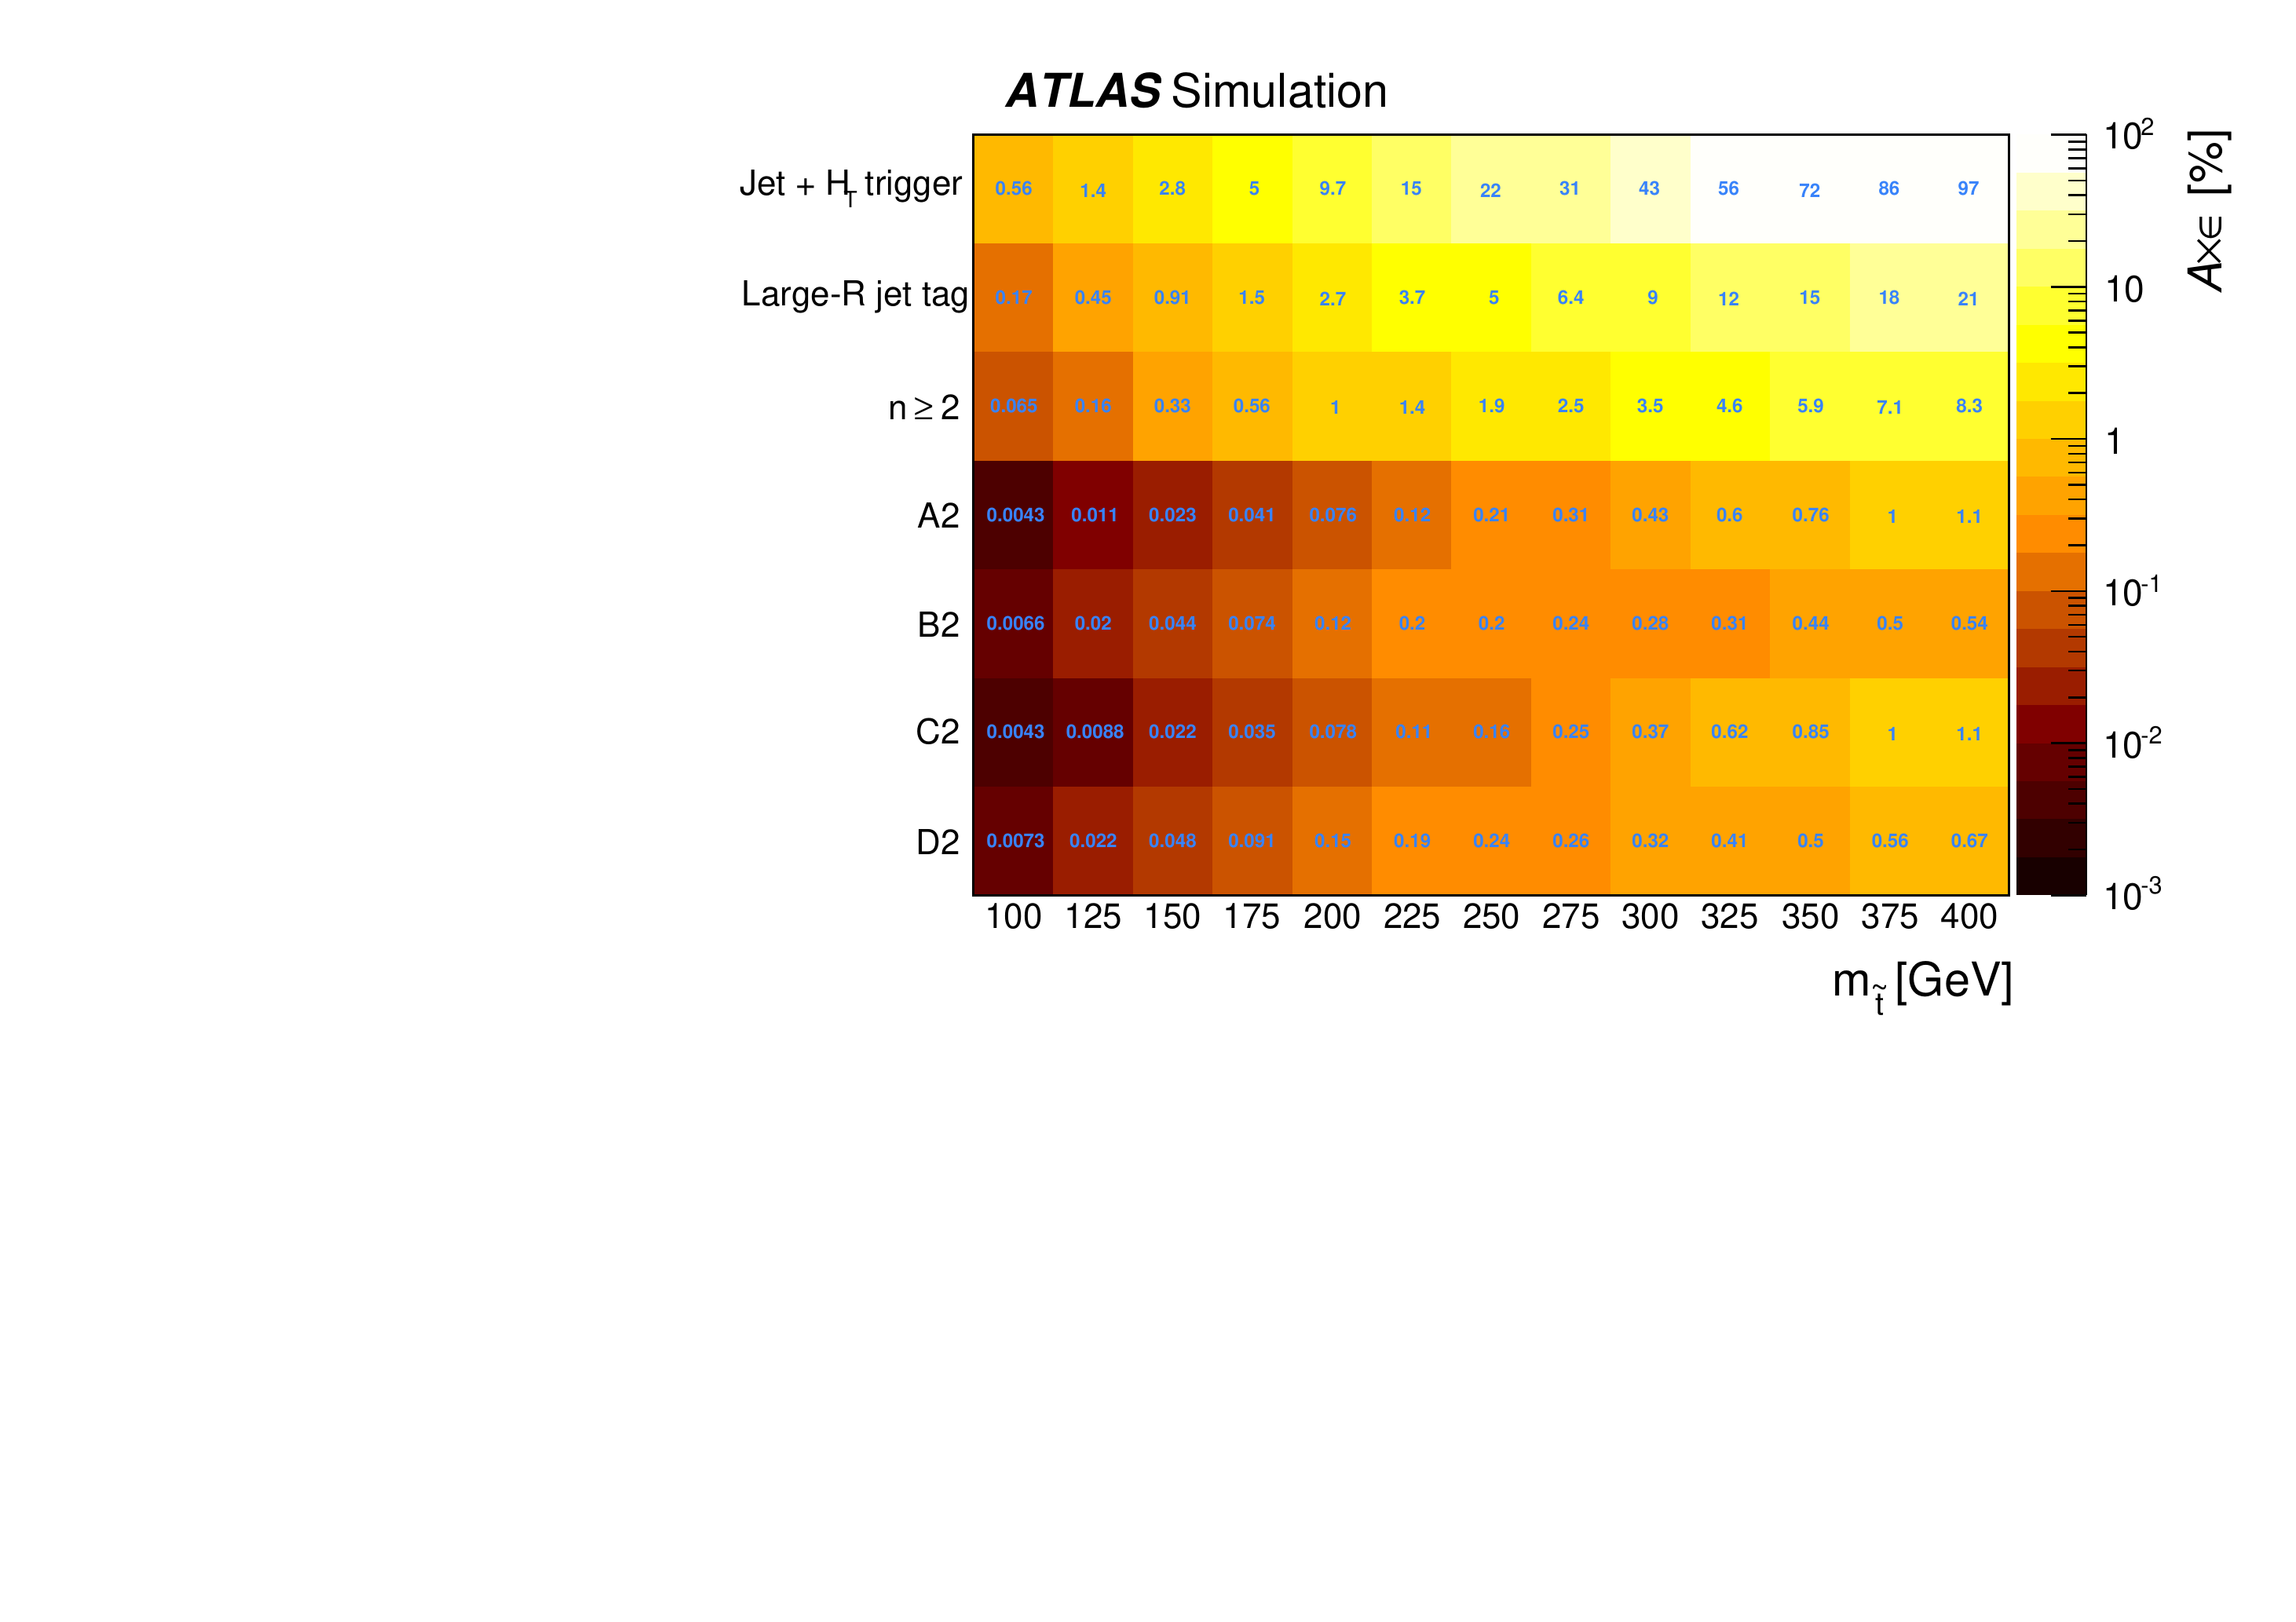}
    \caption{The product of signal acceptance and efficiency ($A\times\epsilon$) with respect to total cross-section as a function of \mstop for each of the selections applied to the $\nbtag\geq2$ region. All numbers are shown as percentages.}
    \label{fig:sigeffvsmass2D}
\end{figure}
%---------------------

\newpage

\subsection{Additional information about signal MC events}
%---------------------
\input{tab-xsect-signal.tex}
%---------------------

\newpage
\FloatBarrier

\subsection{Observed and expected $95\%$ $CLs$}
%---------------------
\input{tab-CLs.tex}
%---------------------

\newpage
\FloatBarrier

\subsection{Shape comparisons of \mavg in all regions}
%%------------------------------    
\begin{figure}[!ht]
  \centering
  \subfigure[Region A]{
    \includegraphics[width=0.48\columnwidth]{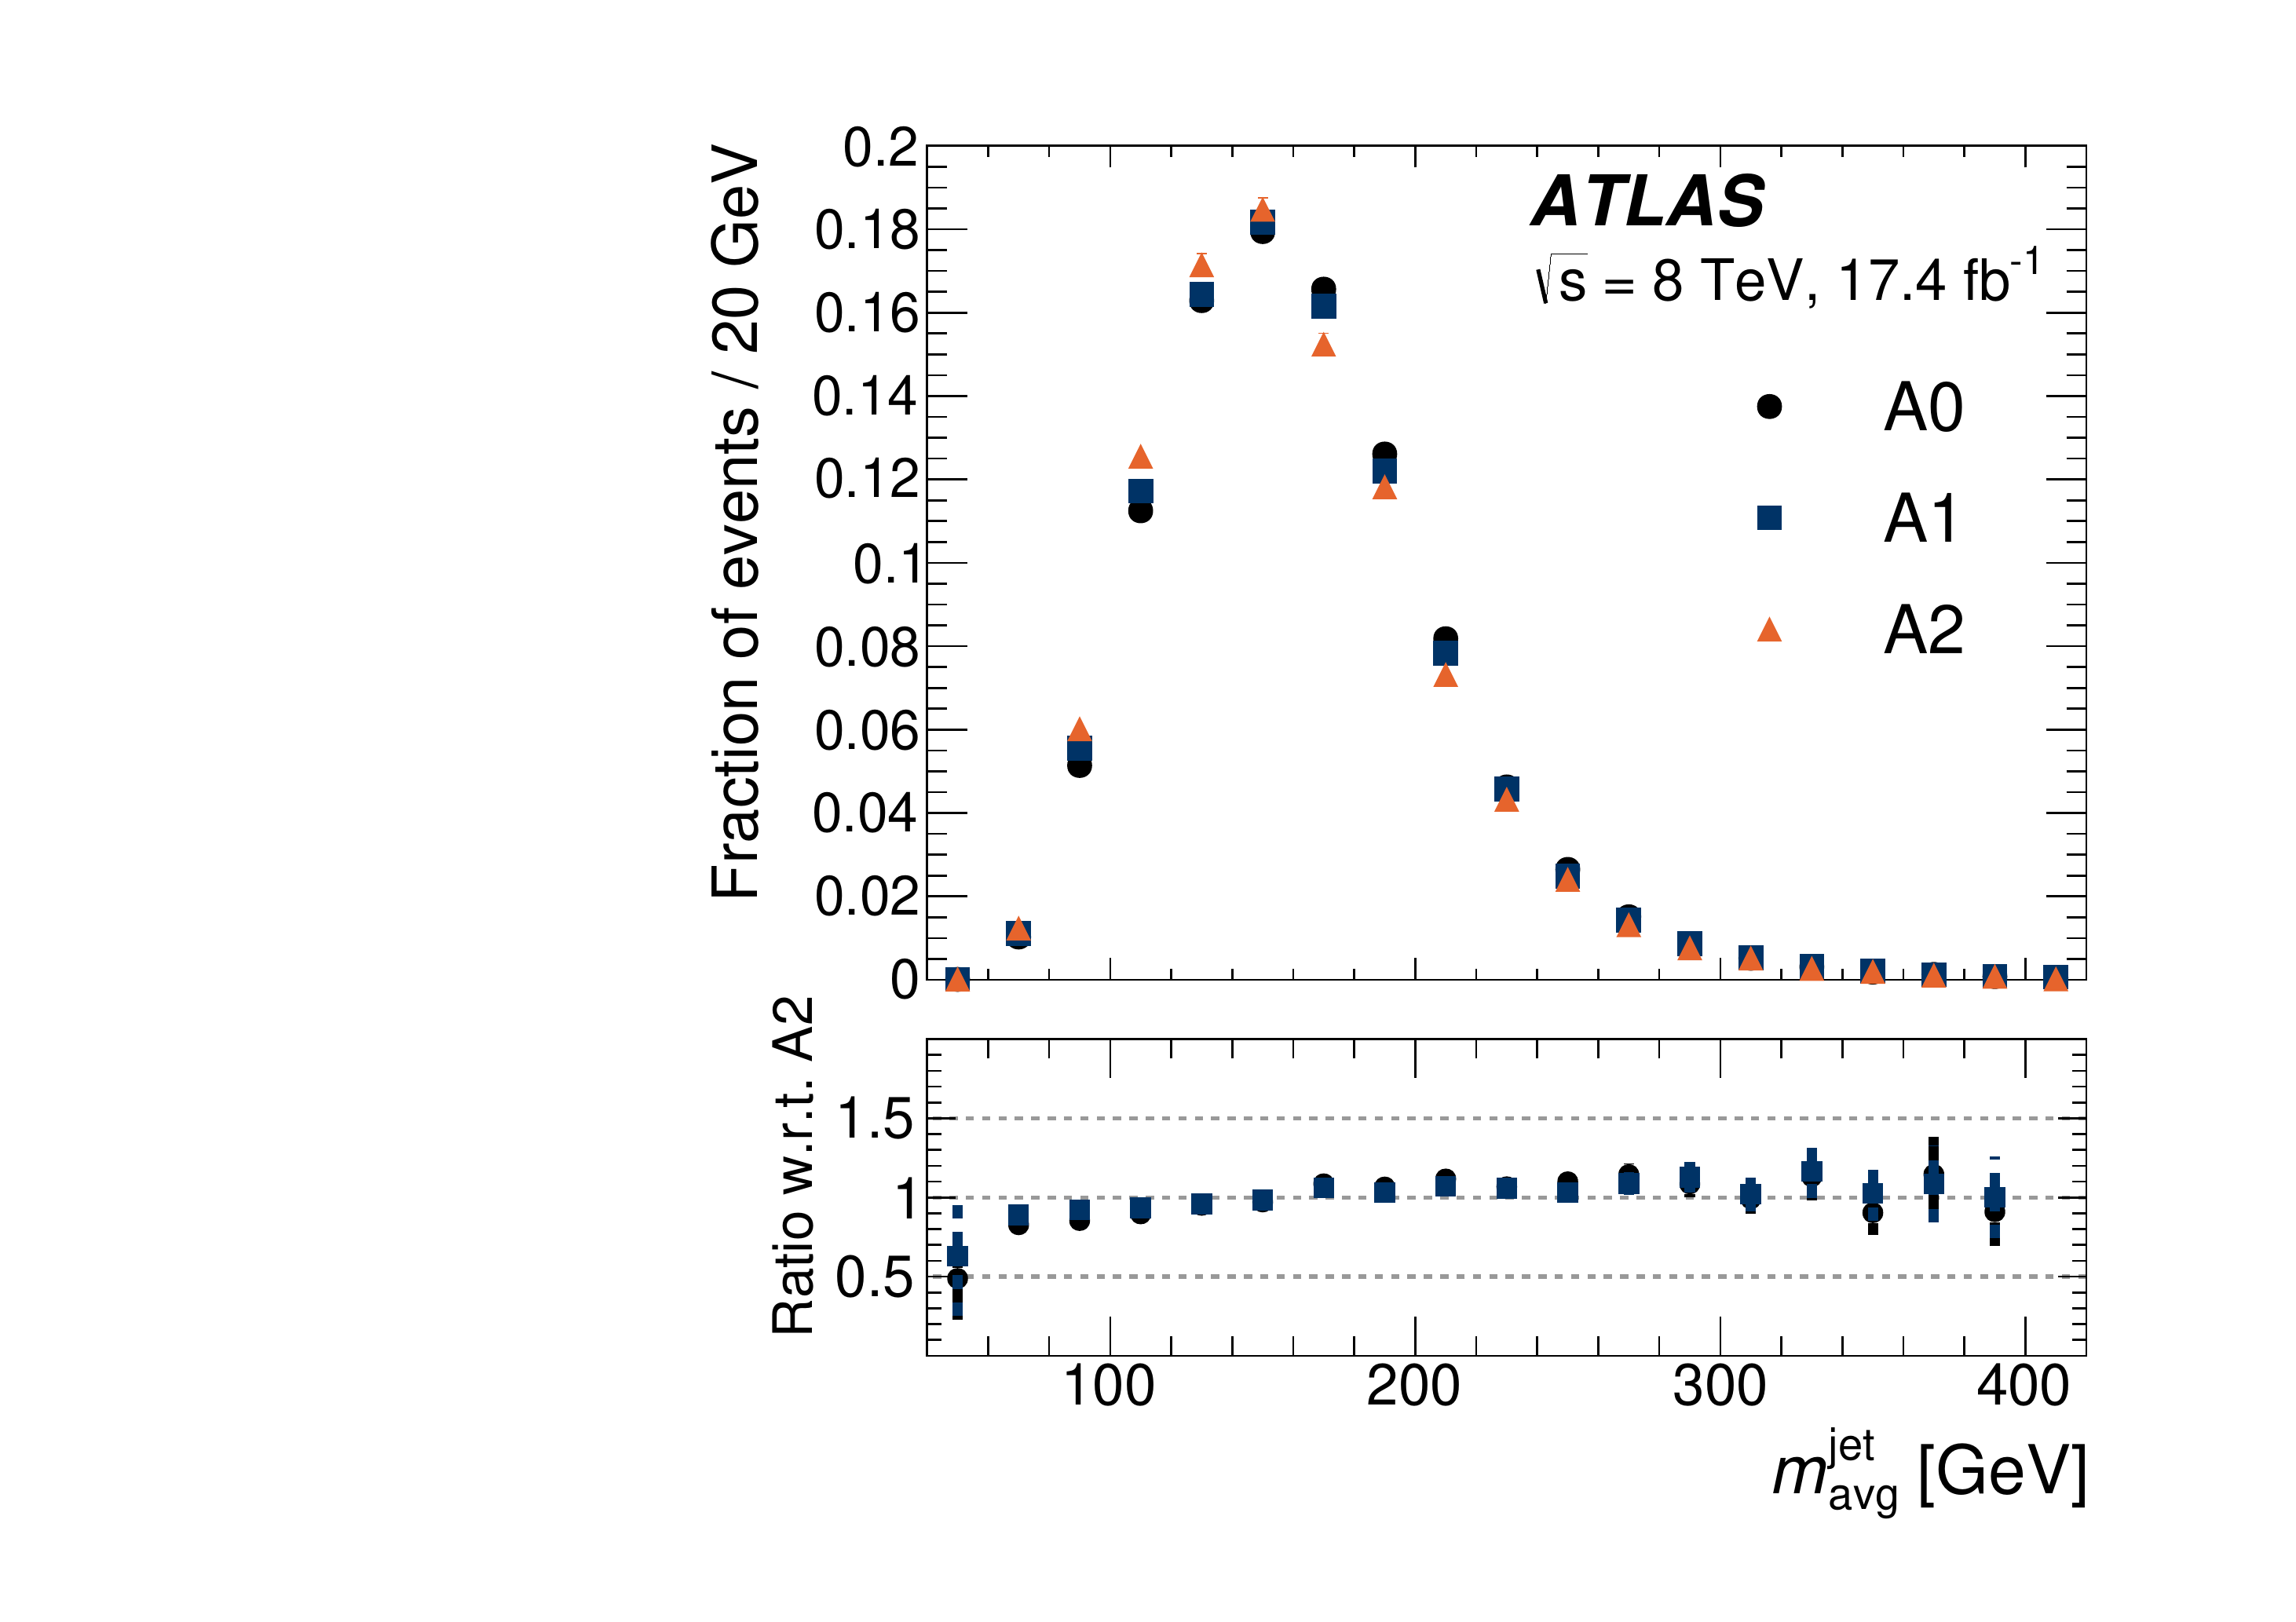}
    \label{fig:app:bckg:sidebands:regionA}
  }
  \subfigure[Region B]{
    \includegraphics[width=0.48\columnwidth]{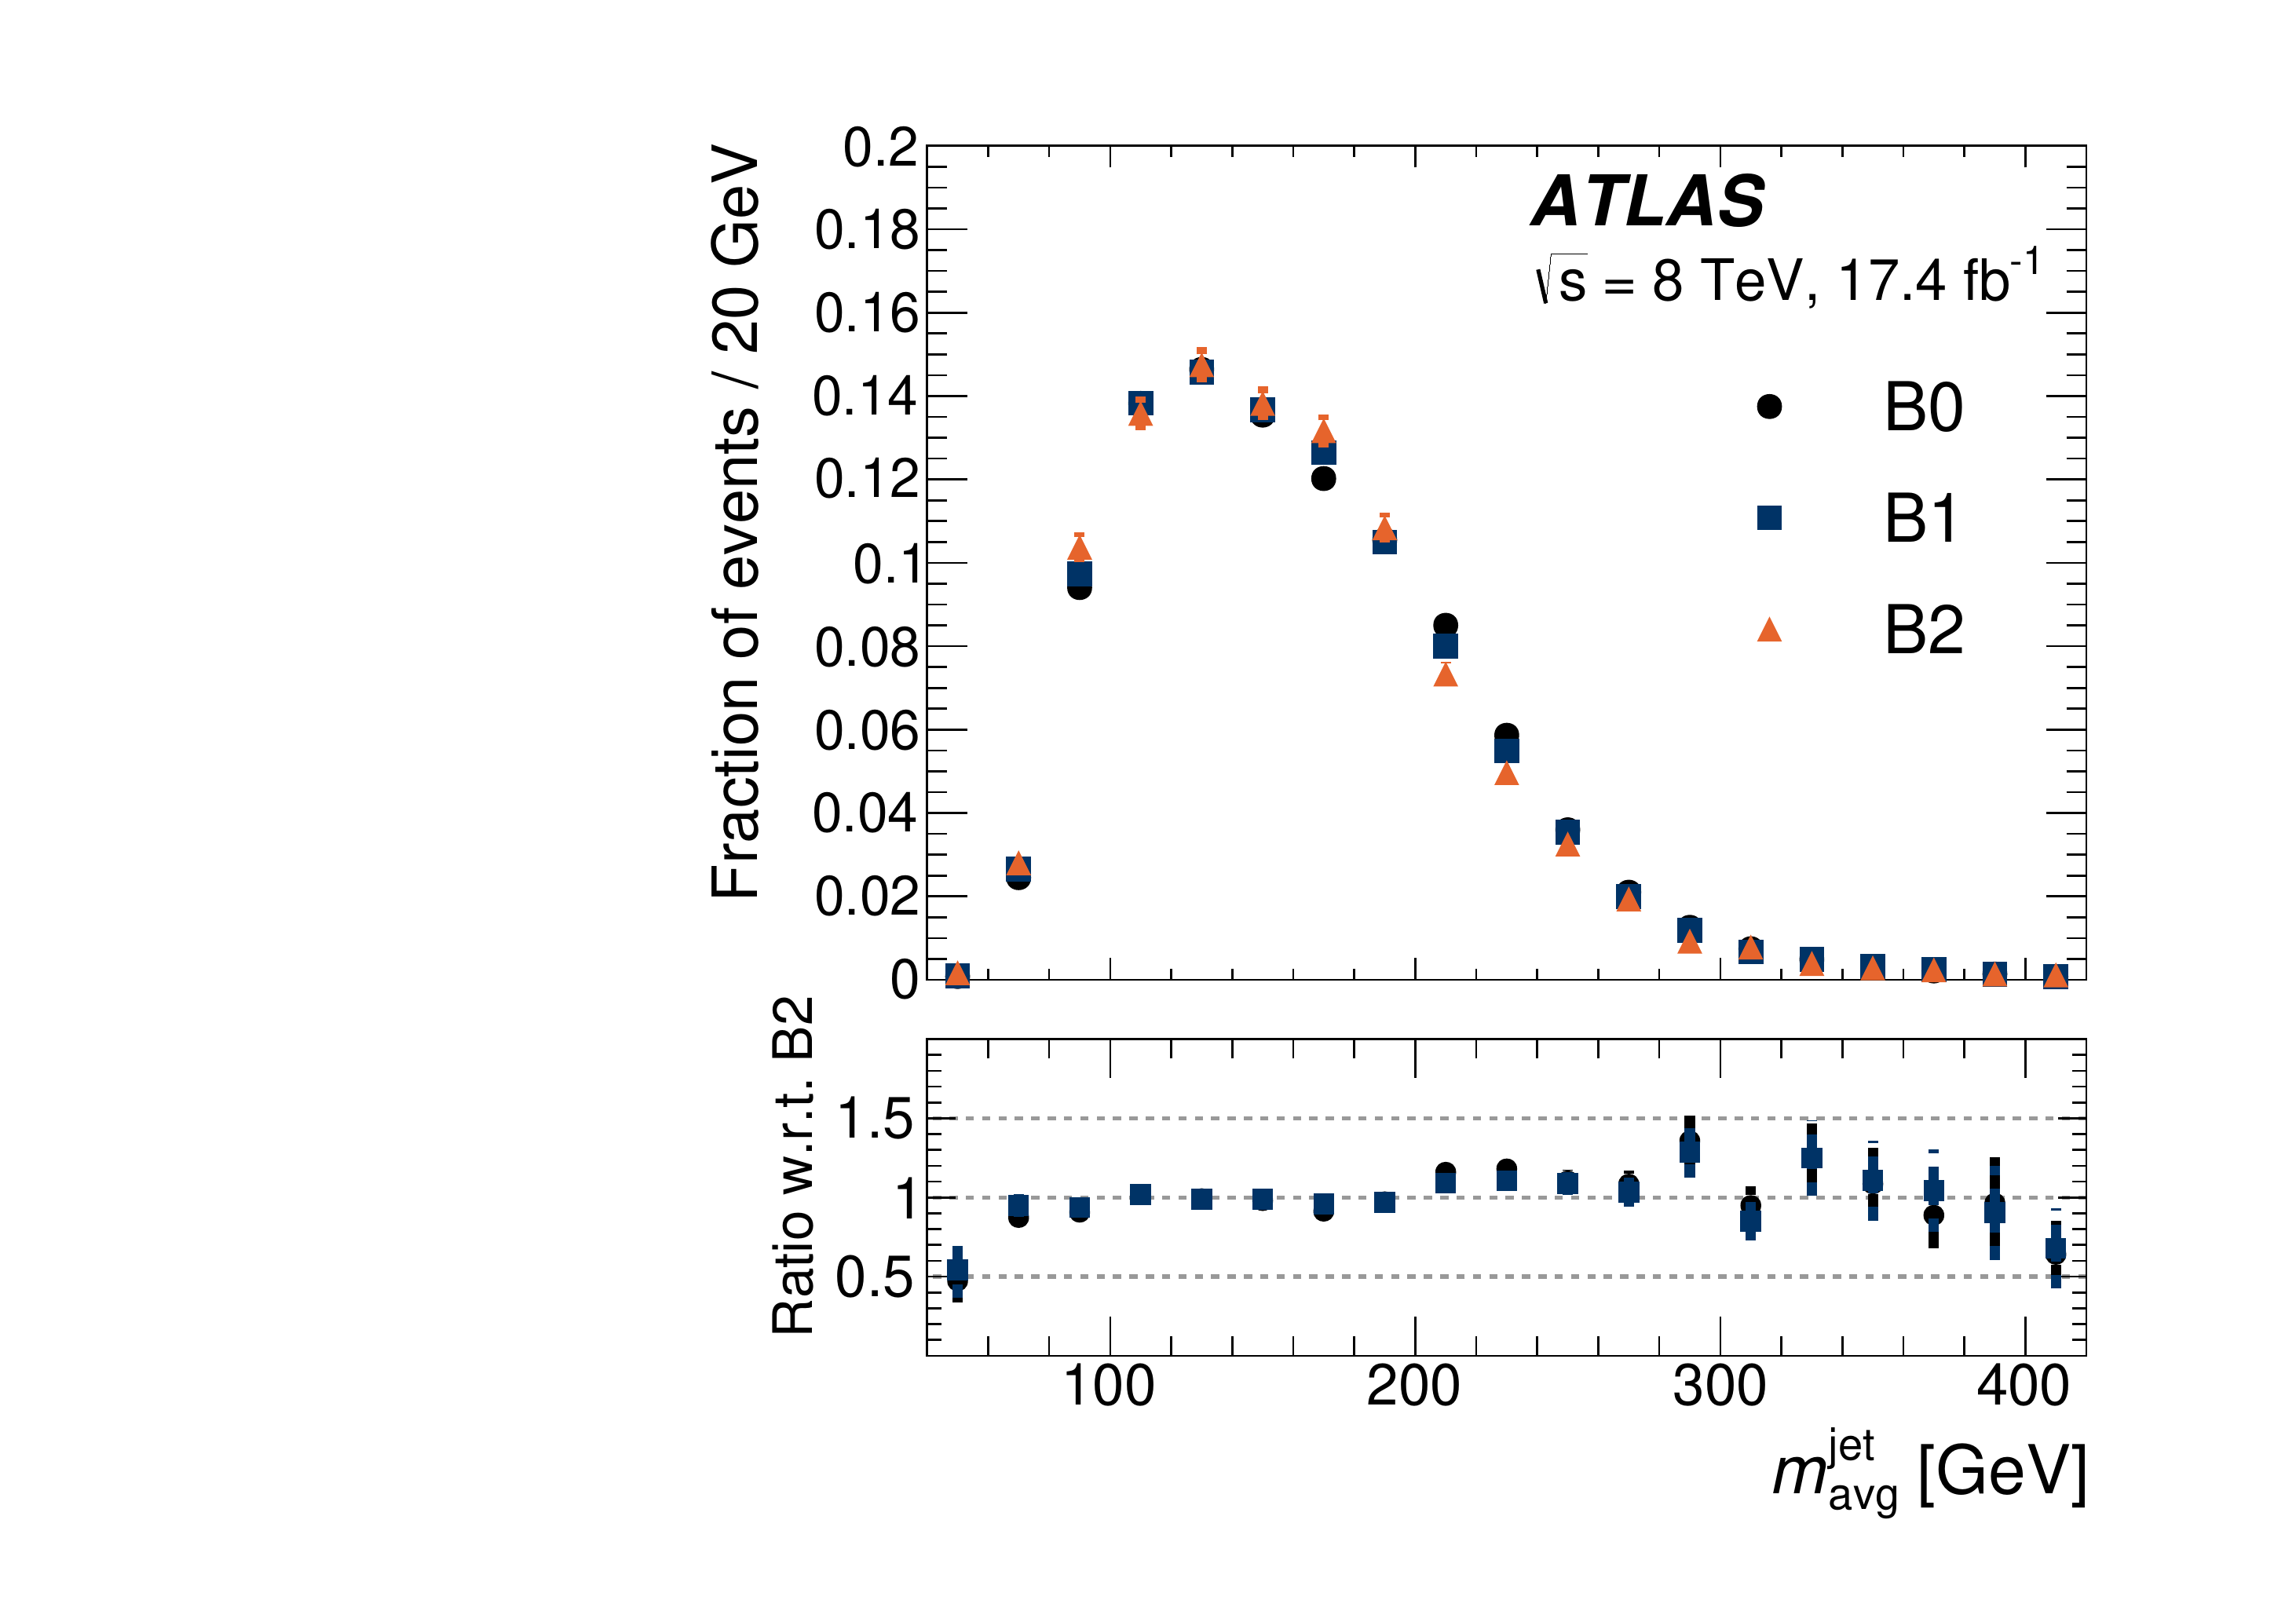}
    \label{fig:app:bckg:sidebands:regionB}
  } \\
    \subfigure[Region C]{
      \includegraphics[width=0.48\columnwidth]{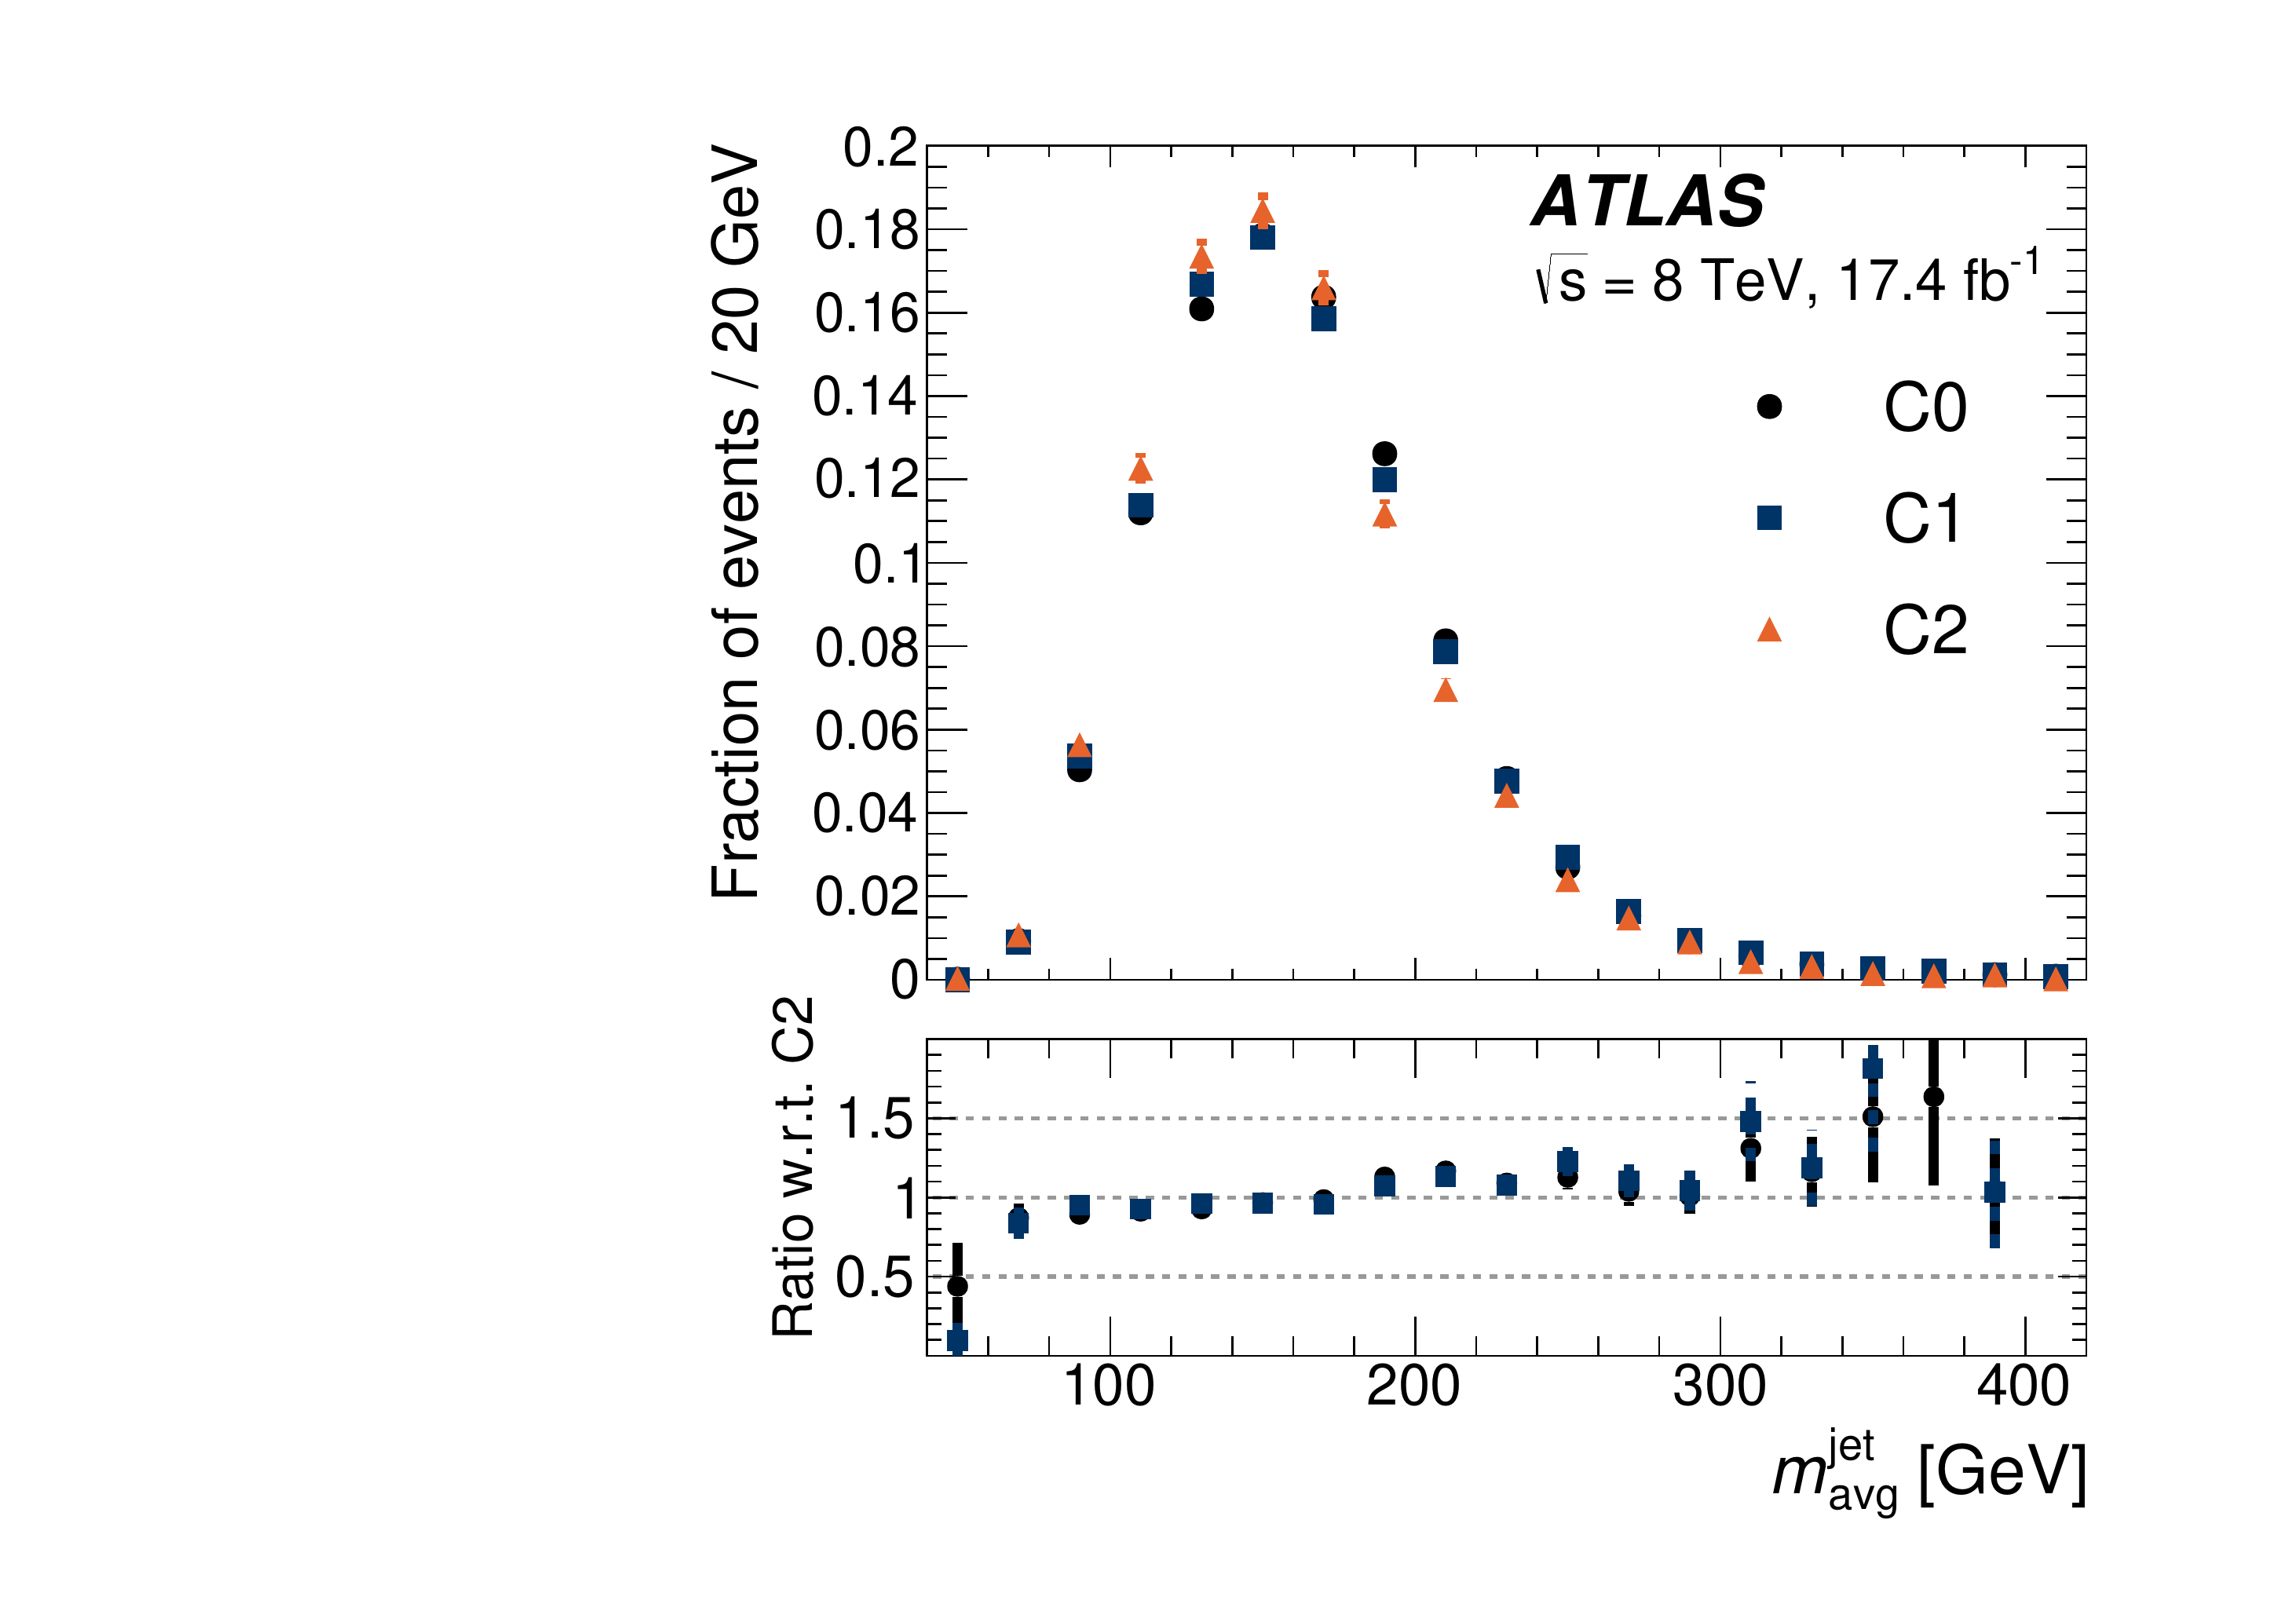}
      \label{fig:app:bckg:sidebands:regionC}
  }
    \subfigure[Region D]{
      \includegraphics[width=0.48\columnwidth]{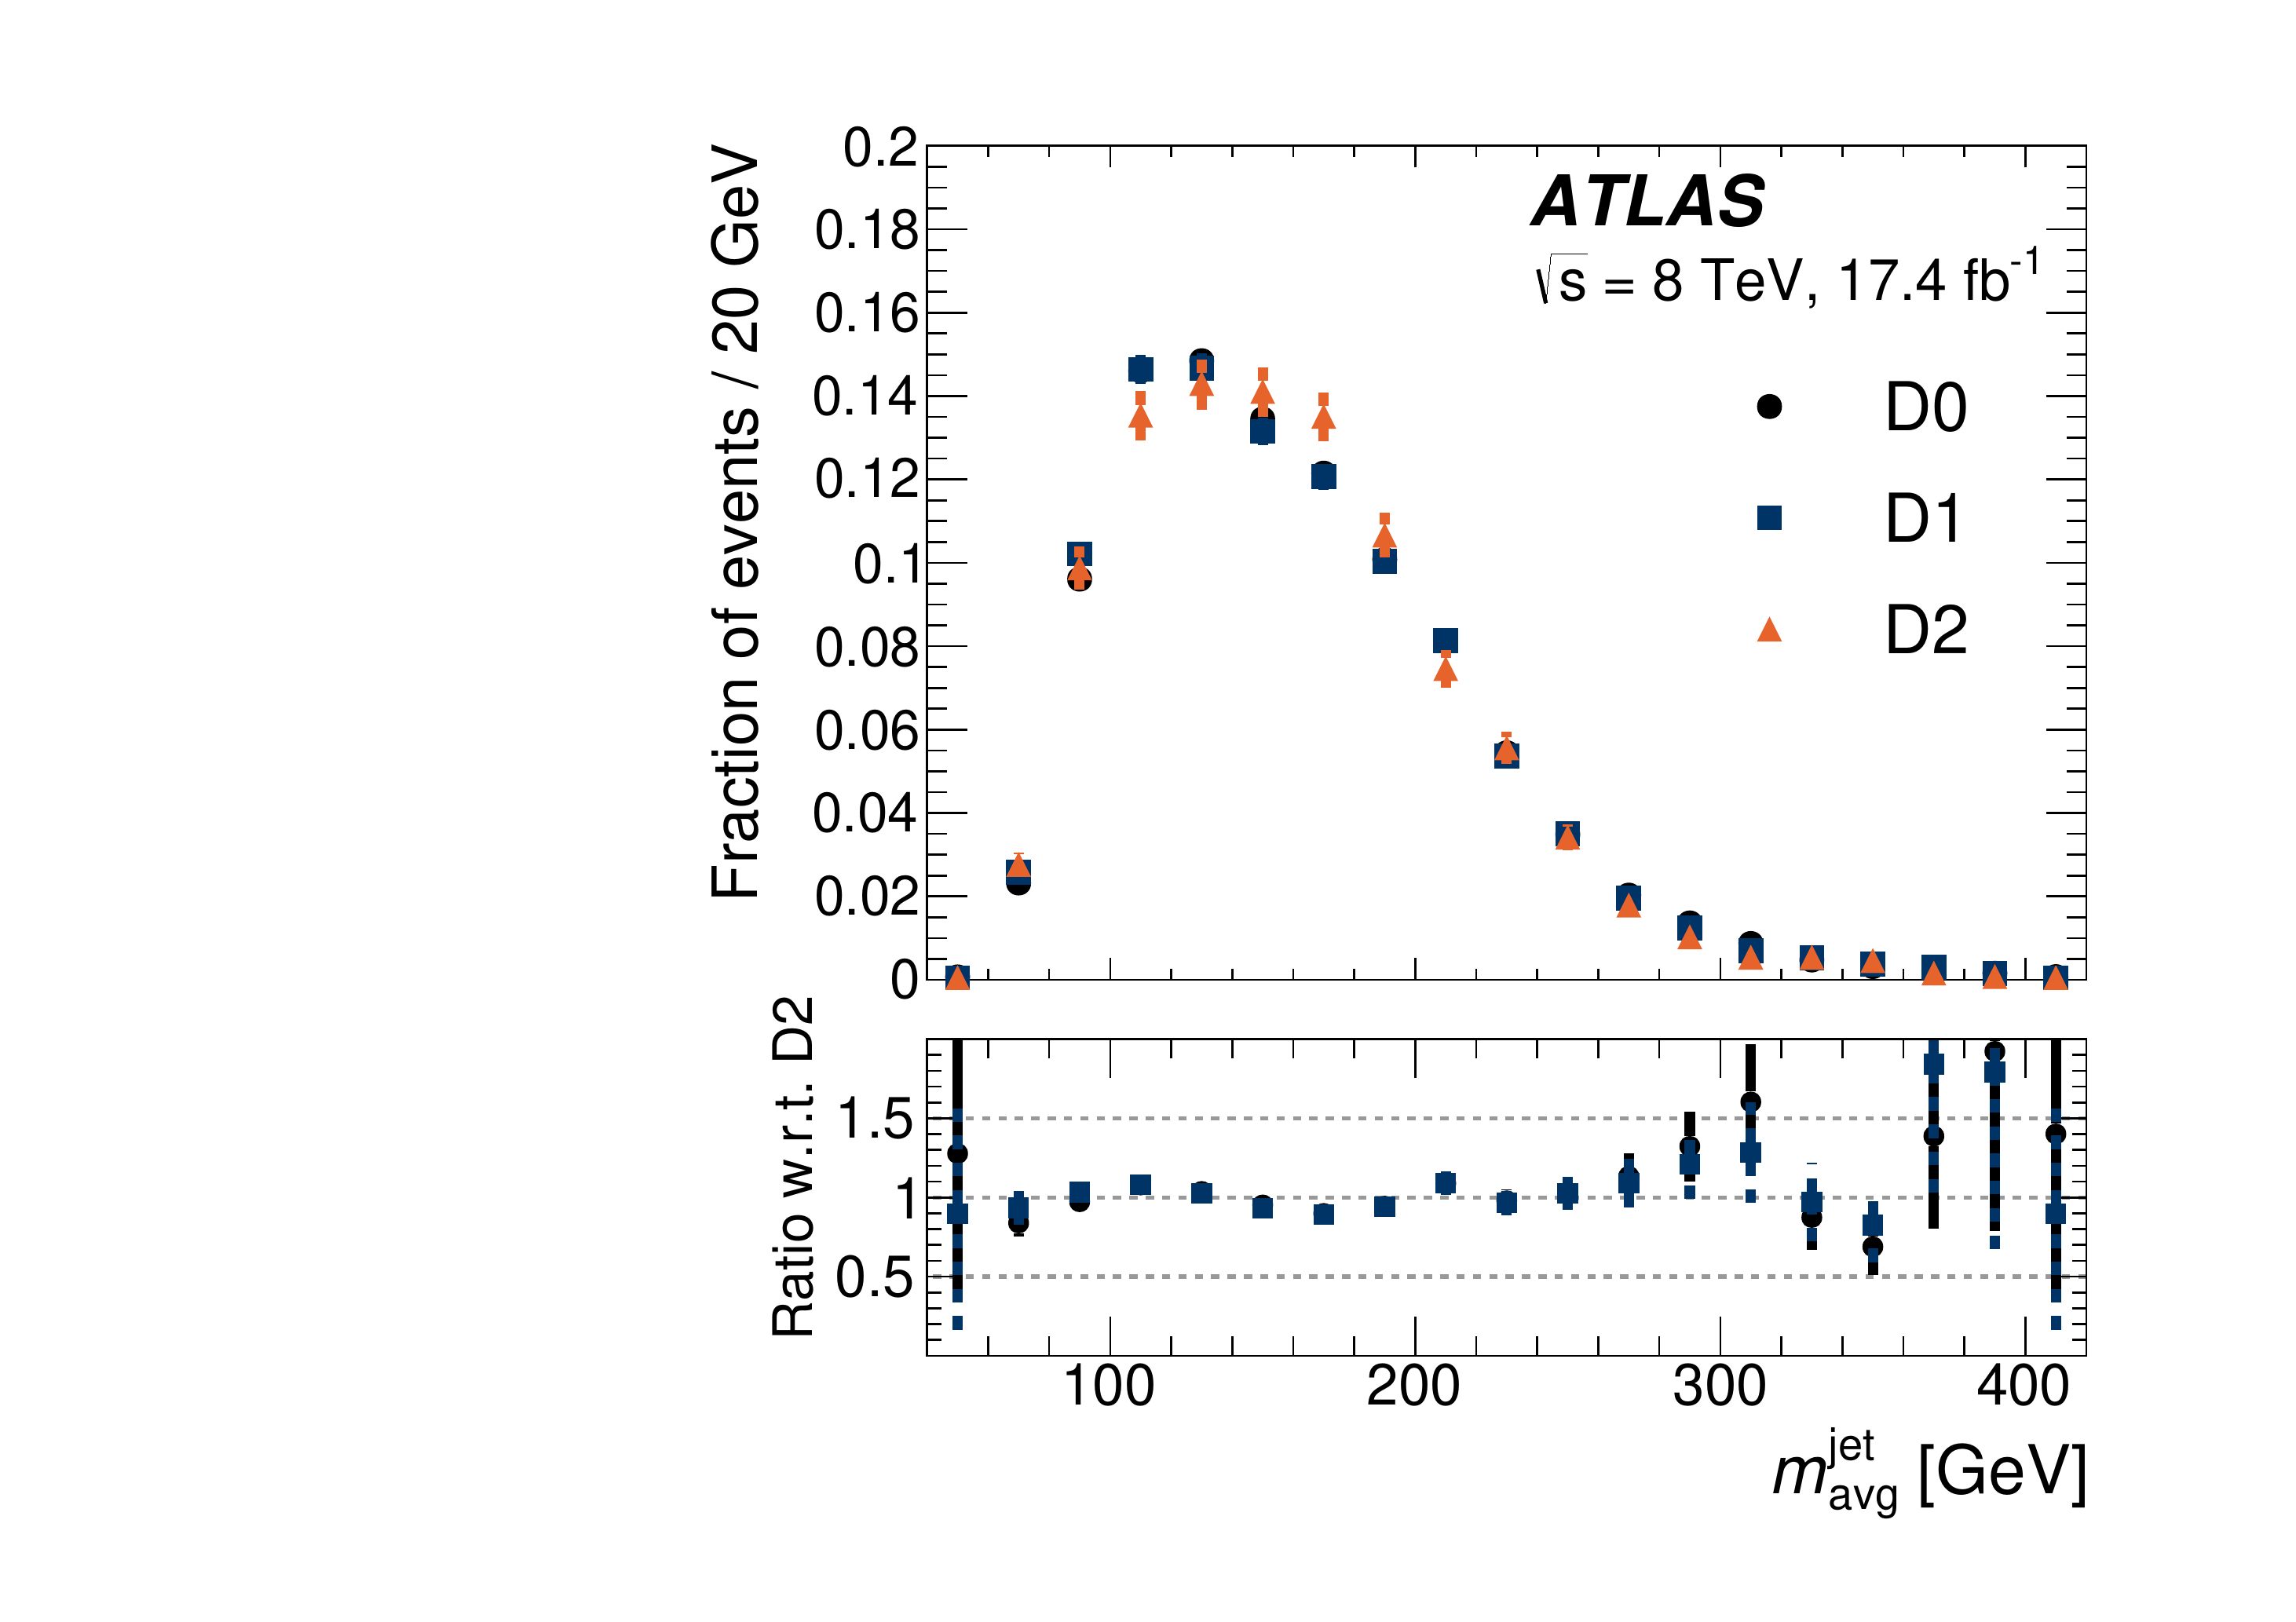}
      \label{fig:app:bckg:sidebands:regionD}
  }~
  \caption{Shape comparisons of the \mavg spectra for events with $\nbtag = 0, = 1, \geq 2$ in regions $A-D$. In each case, the lower panel shows the ratio of each spectrum to the spectrum where $\nbtag\geq2$. Only statistical uncertainties are shown. \label{fig:app:bckg:sidebands}}
\end{figure}
%%------------------------------

\newpage

\subsection{Event displays}

%%------------------------------    
\begin{figure}[!ht]
  \centering
  \subfigure[Data event: \AKT $R=0.4$ jets]{
    \includegraphics[width=0.48\columnwidth]{EventDisplays/rpvStop_data12_AKT4_pT20GeV_fill_2082_etaphi_default.pdf}
    \label{fig:app:display:data:akt4}
  }
  \subfigure[Data event: \AKT $R=1.5$ jets]{
    \includegraphics[width=0.48\columnwidth]{EventDisplays/rpvStop_data12_AKT15_pT100GeV_antiktsubjets_ptfrac_2082_etaphi_default.pdf}
    \label{fig:app:display:data:akt15}
  }
  \caption{Data event with $\mavg = 145$~GeV, $\Asym=0.08$, and $\costhstar=0.26$. The jets displayed are reconstructed using the \AKT algorithm with either $R=0.4$ or $R=1.5$, as indicated in the legend. In cases where \AKT subjets are shown, a radius parameter of $R=0.4$ is used. $R=0.4$ jets are coloured according to their \pt. $R=0.4$ subjets are shaded according to their \pt\ fraction, defined as the ratio of the \pT of the $R=0.4$ subjet to the \pT of the parent $R=1.5$ jet. Only subjets with a \pt\ fraction greater than 10\% are shown. The dots shown represent the topological clusters that are used as input to the jet finding. \label{fig:app:display:data}}
\end{figure}
%%------------------------------

%%------------------------------    
\begin{figure}[!ht]
  \centering
  \subfigure[$\mstop = 100\GeV$: \AKT $R=0.4$ jets]{
    \includegraphics[width=0.48\columnwidth]{EventDisplays/rpvStop_mc12_8TeV_T100_AKT4_pT20GeV_fill_316_etaphi_default.pdf}
    \label{fig:app:display:m100:akt4}
  }
  \subfigure[$\mstop = 100\GeV$: \AKT $R=1.5$ jets]{
    \includegraphics[width=0.48\columnwidth]{EventDisplays/rpvStop_mc12_8TeV_T100_AKT15_pT100GeV_antiktsubjets_ptfrac_316_etaphi_default.pdf}
    \label{fig:app:display:m100:akt15}
  }
  \caption{Signal event ($\mstop = 100\GeV$) with $\mavg = 107$~GeV, $\Asym=0.02$, and $\costhstar=0.13$. The jets displayed are reconstructed using the \AKT algorithm with either $R=0.4$ or $R=1.5$, as indicated in the legend. In cases where \AKT subjets are shown, a radius parameter of $R=0.4$ is used. $R=0.4$ jets are coloured according to their \pt. $R=0.4$ subjets are shaded according to their \pt\ fraction, defined as the ratio of the \pT of the $R=0.4$ subjet to the \pT of the parent $R=1.5$ jet. Only subjets with a \pt\ fraction greater than 10\% are shown. The dots shown represent the topological clusters that are used as input to the jet finding. \label{fig:app:display:m100}}
\end{figure}
%%------------------------------


%%------------------------------    
\begin{figure}[!ht]
  \centering
  \subfigure[$\mstop = 250\GeV$: \AKT $R=0.4$ jets]{
    \includegraphics[width=0.48\columnwidth]{EventDisplays/rpvStop_mc12_8TeV_T250_AKT4_pT20GeV_fill_1751_etaphi_default.pdf}
    \label{fig:app:display:m250:akt4}
  }
  \subfigure[$\mstop = 250\GeV$: \AKT $R=1.5$ jets]{
    \includegraphics[width=0.48\columnwidth]{EventDisplays/rpvStop_mc12_8TeV_T250_AKT15_pT100GeV_antiktsubjets_ptfrac_1751_etaphi_default.pdf}
    \label{fig:app:display:m250:akt15}
  }
  \caption{Signal event ($\mstop = 250\GeV$) with $\mavg = 255$~GeV, $\Asym=0.04$, and $\costhstar=0.17$. The jets displayed are reconstructed using the \AKT algorithm with either $R=0.4$ or $R=1.5$, as indicated in the legend. In cases where \AKT subjets are shown, a radius parameter of $R=0.4$ is used. $R=0.4$ jets are coloured according to their \pt. $R=0.4$ subjets are shaded according to their \pt\ fraction, defined as the ratio of the \pT of the $R=0.4$ subjet to the \pT of the parent $R=1.5$ jet. Only subjets with a \pt\ fraction greater than 10\% are shown. The dots shown represent the topological clusters that are used as input to the jet finding. \label{fig:app:display:m250}}
\end{figure}
%%------------------------------


%%------------------------------    
\begin{figure}[!ht]
  \centering
  \subfigure[$\mstop = 400\GeV$: \AKT $R=0.4$ jets]{
    \includegraphics[width=0.48\columnwidth]{EventDisplays/rpvStop_mc12_8TeV_T400_AKT4_pT20GeV_fill_268_etaphi_default.pdf}
    \label{fig:app:display:m400:akt4}
  }
  \subfigure[$\mstop = 400\GeV$: \AKT $R=1.5$ jets]{
    \includegraphics[width=0.48\columnwidth]{EventDisplays/rpvStop_mc12_8TeV_T400_AKT15_pT100GeV_antiktsubjets_ptfrac_268_etaphi_default.pdf}
    \label{fig:app:display:m400:akt15}
  }
  \caption{Signal event ($\mstop = 400\GeV$) with $\mavg = 385$~GeV, $\Asym=0.07$, and $\costhstar=0.13$. The jets displayed are reconstructed using the \AKT algorithm with either $R=0.4$ or $R=1.5$, as indicated in the legend. In cases where \AKT subjets are shown, a radius parameter of $R=0.4$ is used. $R=0.4$ jets are coloured according to their \pt. $R=0.4$ subjets are shaded according to their \pt\ fraction, defined as the ratio of the \pT of the $R=0.4$ subjet to the \pT of the parent $R=1.5$ jet. Only subjets with a \pt\ fraction greater than 10\% are shown. The dots shown represent the topological clusters that are used as input to the jet finding. \label{fig:app:display:m400}}
\end{figure}
%%------------------------------
